# Supplementary material for: Multi hash embeddings in spaCy
Source: arXiv:2212.09255 source file (2022-12-19)
Supplement: Supplementary file 1 [file appendix.tex]

%\newpage
\begin{comment}
\subsection{Model architecture and training}
\label{sec:architecture}


The named entity recognizer model is a structured prediction approach that falls into the transition-based 
modeling framework popular in syntactic parsing. Most transition-based parsers, including spaCy's 
\texttt{EntityRecognizer}  component, are special cases of bottom-up weighted pushdown automata. They are 
abstract machines that manipulate an input buffer of tokens and a stack of partially constructed structures. 
The \texttt{EntityRecognizer}'s transition system is based on the BILUO sequence encoding scheme. On the stack 
it has zero or one entity currently under construction and zero or more entities that have been previously 
completed. The actions in the transition system are:


\begin{itemize}
    \item Begin-$x$: Open a new entity labelled $x$, initialized with the current word. Advance to the next word. This action is invalid if an entity is currently open.
    \item In-$x$: Add the current word to the currently open entity. Advance to the next word. This action is invalid if there is no entity currently open, or if the current entity does not have the label $x$.
    \item Last-$x$: Add the current word to the currently open entity, and close it. Advance to the next word. This action is invalid if there is no entity currently open, or if the current entity does not have the label $x$.
    \item Unit-$x$: Open a new entity labelled $x$, consisting of the current word. Close the entity. Advance to the next word. This action is invalid if an entity is currently open.
    \item Out: Advance to the next word. This action is invalid if an entity is currently open.
\end{itemize}


The named entity recognizer makes these decisions based on the state-representations which consist of three 
tokens: the current word, the first word of the current entity (if one is open), and the last word of the 
current entity (if one is open) and three additional context tokens, representing additional words from the 
currently open entity, if they are present. A feed-forward network computes a state vector given the state's 
contextual features and another feed-forward network computes the action scores from the state vector.

The state representation network is a single-layer Maxout network with the $hidden\_width$ of 64 
and the default number of context tokens for the state (i.e., 8), the maxout layer will have an input width of 512. 
The maxout layer uses two pieces by default, which means it will have an output width of 128 
($maxout\_pieces * hidden\_width$). The state vector will then be reduced down to a width of 64 after the 
maxout nonlinearity. The action prediction layer is a single linear layer, followed by a softmax activation. 

We use a dynamic oracle for the transition system in order to train the model 
with an imitation learning objective. To define the dynamic oracle, we consider the ``score'' of an analysis 
to be $-{FP} + -{FN}$, where $FP$ is the number of false-positive entities in the analysis, and $FN$ is the 
number of false-negative entities. An analysis that includes all of the correct entities and no incorrect 
entities will receive a score of 0, the optimal score. Actions that open an incorrect entity or cause a 
correct entity to be unrecoverable will reduce the optimal reachable score, and therefore marked incorrect.


\begin{figure}[t]
    \centering
    \includegraphics[width=0.85\textwidth]{figures/pushdown_automata.pdf}
    \caption{Performance of  \texttt{MultiHashEmbed} with different number of seeds. Evaluated on the development set.}
    \label{fig:pushdown}
\end{figure}

Notably, this objective is defined in terms of \emph{entities}, rather than \emph{tokens}. This becomes 
relevant once a mistake has been made, and the parser enters a configuration where an entity is open that is 
known to be incorrect (it may have been started in the wrong place, or extended past its correct ending). The 
scoring system is indifferent to where such incorrect entities should be ended, so long as they are not 
extended so far that they make a correct entity unrecoverable. Whether an incorrect entity consists of 2 
tokens or 10, it will still be scored as one incorrect entity. Instead of this flexible objective, 
we could insist that if the current entity is incorrect, the only correct action is to end it immediately. 
However, this would make it likely that the parser will sometimes end a \emph{correct} entity early, if it 
suddenly guesses it might be incorrect.






%This algorithm has structural features that make it well-suited to named entity recognition problems, 
%especially in languages similar to English. However, it may be less well suited to the recognition of 
%arbitrary spans that do not represent named entities. In languages similar to English, named entities 
%generally have distinct boundary tokens. Our named entity recognition algorithm relies on this, especially 
%since it processes the sentence left-to-right, with greedy search. This can be expected to perform poorly 
%on problems where the word that gives away the span's label occurs somewhere in the middle or to the end. 
%Given a sufficiently powerful token-to-vector encoding, such as a transformer model, the algorithm may still be 
%able to learn these problems effectively, but it can be expected to be at a disadvantage. The structure of the 
%loss may also be problematic in some span identification tasks. In some span tasks, the borders of the span 
%are not especially important, and partial overlap should receive partial credit. We plan to introduce a 
%separate component that will be better suited to the recognition of arbitrary spans that are not named 
%entities.
\end{comment}
